# Supplementary material for: DWR-Drag: A new generation software for the Double Wall-Ring Interfacial Shear Rheometer's data analysis
Source: arXiv:2408.15755 source file (2024-08-28)
Supplement: Supplementary file 1 [file CPC_DWR_Suppl_Mat.pdf]

# Supplementary Materials for Improved data processing for the Double Wall-Ring Interfacial Shear Rheometer

Pablo Sanchez-Puga[a,b,*], Miguel. A. Rubio[b]

[a] *Institut Laue-Langevin, 38042, Grenoble (France)*
[b] *Departamento de Física Fundamental, Facultad de Ciencias, Universidad Nacional de Educación a Distancia (UNED), 28232, Las Rozas (Spain)*

---

---

## 1. Mathematical expressions for the boundary conditions

In terms of the amplitude functions, $g^*_{(1,2,s)}(r, z)$, the boundary conditions at the solid walls are the following,

$$\begin{aligned} &g_1^*(\bar{R}_1, 0 \leq \bar{z} \leq \bar{H}) = g_2^*(\bar{R}_2, \bar{H} \leq \bar{z} \leq 2\bar{H}) \\ &= g_1^*(\bar{R}_3, 0 \leq \bar{z} \leq \bar{H}) = g_2^*(\bar{R}_4, \bar{H} \leq \bar{z} \leq 2\bar{H}) = 0, \end{aligned} \quad (1)$$

on the half-height steps and at the bottom wall,

$$g_2^*(\bar{R}_2 \leq \bar{r} \leq \bar{R}_1, \bar{H}_1) = g_2^*(\bar{R}_3 \leq \bar{r} \leq \bar{R}_4, \bar{H}_1) = g_1^*(\bar{R}_1 \leq \bar{r} \leq \bar{R}_3, 0) = 0, \quad (2)$$

at the DWR lower inner surface,

$$g_1^*(\bar{R}_5 \leq \bar{r} \leq \bar{R}_r, \bar{z} = \bar{H}_1 + \frac{\bar{H}_r(\bar{r} - \bar{R}_5)}{\bar{R}_5 - \bar{R}_r} : \bar{H}_1 - \bar{H}_r \leq \bar{z} \leq \bar{H}_1) = \frac{\bar{r}}{\bar{R}_6}, \quad (3)$$

at the DWR lower outer surfaces,

$$g_1^*(\bar{R}_r \leq \bar{r} \leq \bar{R}_6, \bar{z} = \bar{H}_1 - \bar{H}_r - \frac{\bar{H}_r(\bar{r} - \bar{R}_r)}{\bar{R}_r - \bar{R}_6} : \bar{H}_1 - \bar{H}_r \leq \bar{z} \leq \bar{H}_1) = \frac{\bar{r}}{\bar{R}_6}, \quad (4)$$

*Corresponding author.
*E-mail address:* sanchez-puga@ill.fr

at the DWR upper inner surface,

$$g_2^*(\bar{R}_5 \leq \bar{r} \leq \bar{R}_r, \bar{z} = \bar{H}_1 - \frac{\bar{H}_r(\bar{r}-\bar{R}_5)}{\bar{R}_r - \bar{R}_5} : \bar{H}_1 \leq \bar{z} \leq \bar{H}_1 + \bar{H}_r) = \frac{\bar{r}}{\bar{R}_6}, \tag{5}$$

at the DWR upper outer surface,

$$g_2^*(\bar{R}_r \leq \bar{r} \leq \bar{R}_6, \bar{z} = \bar{H}_1 + \bar{H}_r + \frac{\bar{H}_r(\bar{r}-\bar{R}_r)}{\bar{R}_6 - \bar{R}_r} : \bar{H}_1 \leq \bar{z} \leq \bar{H}_1 + \bar{H}_r) = \frac{\bar{r}}{\bar{R}_6}, \tag{6}$$

at the upper bulk phase top surface in the free surface approximation,

$$\left.\frac{\partial g_2^*}{\partial \bar{z}}\right|_{\bar{R}_2 < \bar{r} < \bar{R}_4, \bar{z} = \bar{H}_1 + \bar{H}_2} = 0, \tag{7}$$

and at the upper bulk phase top surface in the no slip approximation,

$$g_2^*(\bar{R}_2 < \bar{r} < \bar{R}_4, \bar{z} = \bar{H}_1 + \bar{H}_2) = 0, \tag{8}$$

## 2. Detailed expressions of the hydrodynamic drags

$$M_1^* = -i\omega 2\pi\theta_0 e^{i\omega t} R_6^3 \eta_1^* \left( \int_{\bar{R}_5}^{\bar{R}_r} \bar{r}^2 \frac{\partial g_1^*}{\partial \bar{p}_1} d\bar{r} + \int_{\bar{R}_r}^{\bar{R}_6} \bar{r}^2 \frac{\partial g_1^*}{\partial \bar{p}_2} d\bar{r} \right), \tag{9}$$

$$M_2^* = -i\omega 2\pi\theta_0 e^{i\omega t} R_6^3 \frac{\eta_1^*}{Y} \left( \int_{\bar{R}_5}^{\bar{R}_r} \bar{r}^2 \frac{\partial g_2^*}{\partial \bar{p}_3} d\bar{r} + \int_{\bar{R}_r}^{\bar{R}_6} \bar{r}^2 \frac{\partial g_2^*}{\partial \bar{p}_4} d\bar{r} \right), \tag{10}$$

$$M_s^* = i\omega 2\pi\theta_0 e^{i\omega t} R_6^3 \eta_1^* N^* \left( {\bar{R}_5}^3 \frac{\partial}{\partial \bar{r}} \left(\frac{g_s^*}{\bar{r}}\right)\bigg|_{\bar{r}=\bar{R}_5} - \frac{\partial}{\partial \bar{r}} \left(\frac{g_s^*}{\bar{r}}\right)\bigg|_{\bar{r}=\bar{R}_6} \right), \tag{11}$$

where $p_1$, $p_2$, $p_3$, and $p_4$ represent coordinates normal to the faces of the ring's cross-section and the top bars indicate that they are made nondimensional by

dividing by $R_6$. one obtains an expression that relates the complex amplitude ratio, $AR^* = \frac{M_0}{\theta_0} e^{-i\delta}$, to the spatial parts of the drag torques and the inertia term, namely,

$$
\begin{aligned}
AR^* = i\omega 2\pi R_6^3 \eta_1^* & \left[ \left( \int_{\bar{R}_5}^{\bar{R}_r} \bar{r}^2 \frac{\partial g_1^*}{\partial \bar{p_1}} \, d\bar{r} + \int_{\bar{R}_r}^{\bar{R}_6} \bar{r}^2 \frac{\partial g_1^*}{\partial \bar{p_2}} \, d\bar{r} \right) \right. \\
& + \frac{1}{Y} \left( \int_{\bar{R}_5}^{\bar{R}_r} \bar{r}^2 \frac{\partial g_2^*}{\partial \bar{p_3}} \, d\bar{r} + \int_{\bar{R}_r}^{\bar{R}_6} \bar{r}^2 \frac{\partial g_2^*}{\partial \bar{p_4}} \, d\bar{r} \right) \\
& \left. - N^* \left( \bar{R_5}^3 \frac{\partial}{\partial \bar{r}} \left( \frac{g_s^*}{\bar{r}} \right) \bigg|_{\bar{r}=\bar{R}_5} - \frac{\partial}{\partial \bar{r}} \left( \frac{g_s^*}{\bar{r}} \right) \bigg|_{\bar{r}=\bar{R}_6} \right) \right] - I\omega^2. \qquad (12)
\end{aligned}
$$

## 3. Detailed expressions of the discretization scheme

In the above-mentioned approximation, the flow field is fully described by the value of the complex function $g^*(\bar{r}, \bar{z})$ at the mesh nodes. Hence, in the mesh we will have

$$
\begin{aligned}
& g_{j,k}^{1*} = g^{1*} \left( \bar{R}_2 + (j-1)\Delta\bar{s},\, 2\bar{h} - (k-1)\,\Delta\bar{s} \right), \qquad (13) \\
& \forall j, k \in \mathbb{Z}/1 \le j \le N_1 + 1, 1 \le k \le M + 1.
\end{aligned}
$$

$$
\begin{aligned}
& g_{j,k}^{2*} = g^{2*} \left( \bar{R}_1 + (j-1)\Delta\bar{s},\, 2\bar{h} - (k-1)\,\Delta\bar{s} \right), \qquad (14) \\
& \forall j, k \in \mathbb{Z}/1 \le j \le N_2 + 1, M + 2 \le k \le 2M + 1.
\end{aligned}
$$

where $\Delta\bar{s} = \frac{\Delta s}{R_6}$ is the non-dimensional mesh size and $j, k$ the radial and vertical indexes[1]. As mentioned above, the resolution is set by $N_d$ and the ring width, $R_6 - R_5$. Therefore[2]:

---

[1]The code is originally written in MATLAB, consequently, all indices start at 1. In the Python version the range of the indices starts at 0.

[2]Here the brackets, $[\cdot]$, stand for the nearest integer. MATLAB/Python ‘round’ functions are used.

$$\Delta s = \frac{R_6 - R_5}{N_d} \tag{15}$$

$$N_{step} = \left\lceil \frac{R_4 - R_3}{\Delta s} \right\rceil \tag{16}$$

$$N_{G1} = \left\lceil \frac{R_5 - R_1}{\Delta s} \right\rceil \tag{17}$$

$$N_{G2} = \left\lceil \frac{R_3 - R_6}{\Delta s} \right\rceil \tag{18}$$

$$M = \left\lceil \frac{H}{\Delta s} \right\rceil \tag{19}$$

$$N_1 = N_{G1} + N_{G2} + N_d + 2N_{step} \tag{20}$$

$$N_2 = N_{G1} + N_{G2} \tag{21}$$

$$\tag{22}$$

## 4. Illustrative examples of flow fields

In this section we illustrate some examples of the typical flow configurations corresponding to the solutions obtained for the hydrodynamic flow fields both in the bulk fluid phases and at the interface. All of the results here shown correspond to air/water interfaces sheared at $\omega = 1$ rad/s, and have been obtained using a free surface boundary condition at the top of the upper bulk fluid layer, and a spatial resolution, `ringSubs` = 40. The geometrical configuration corresponds to a medium size system with the geometrical parameters indicated in Table 2 of the main text.

### *4.1. Bulk phases flow fields*

First, we show, in Figure 1, the results obtained for a clean air/water interface. Remark that the flow appears to be rather symmetric at left and right of the ring and that the color scale for the in-phase (real) part of the velocity amplitude function spans a much larger range of values than the out-of-phase (imaginary) part. Interestingly, the flow induced by the probe motion penetrates more in the air phase than in the water subphase. This can be understood in terms of expression (15) of the main text and the kinematic viscosity of air ($15.34 \times 10^{-6}$ $\mathrm{m}^2 s^{-1}$, at 23 °C) being larger than the water

one ($9.33 \times 10^{-7}$ m$^2 s^{-1}$, at 23 °C); hence, the momentum decay length in air is approximately four times larger than in water.

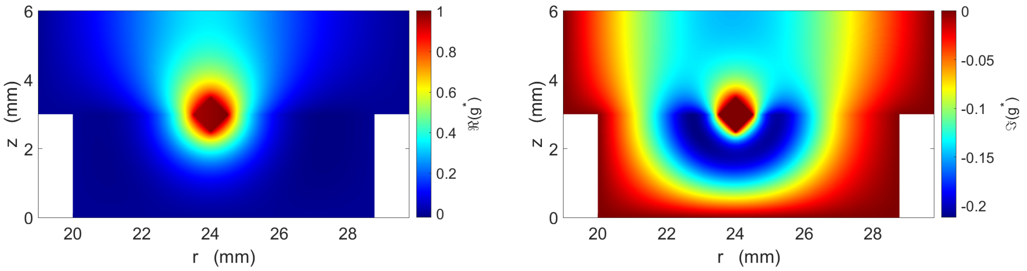


Figure 1: Color coded plot of the flow field at both bulk fluid phases for a clean air/water interface $\eta_s = 0$ Ns/m ($Bq = 0$) at $\omega = 1$ rad/s. Plots at left and right show the in-phase and out-of-phase parts of the velocity amplitude function, respectively.

In Figure 2 we show the results regarding a purely viscous air/water interface, with an interfacial viscosity, $\eta_s = 10^{-5}$ Ns/m ($Bq = 14$). Some small asymmetry of the flow at left and right of the ring is already appreciable. Here, the flow induced by the probe motion penetrates deeply in the air phase while in the water subphase, the in-phase part shows non zero values only in a shallow layer below the interface, and the out-of-phase part attains its maximum value roughly at the center of the subphase.

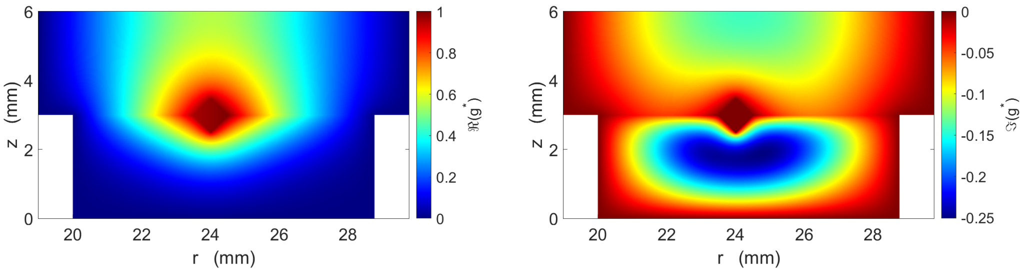


Figure 2: Color coded plot of the flow field at both bulk fluid phases for a purely viscous air/water interface, with interfacial viscosity $\eta_s = 10^{-5}$ Ns/m ($Bq = 14$), at $\omega = 1$ rad/s. Plots at left and right show the in-phase and out-of-phase parts of the velocity amplitude function, respectively.

In Figure 3 we show the results regarding a purely elastic air/water interface, with an interfacial viscosity, $\eta_s^* = -10^{-5} i$ Ns/m ($Bq^* = -14i$) . A

stronger asymmetry of the flow at left and right of the ring is clearly visible. Again, the flow induced by the probe motion penetrates deeply in the air phase while in the water subphase it constitutes a shallow flow below the interface.

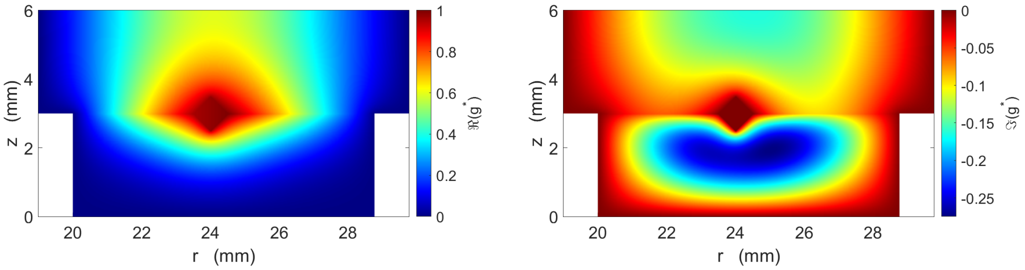


Figure 3: Color coded plot of the flow field at both bulk fluid phases for a purely elastic air/water interface, with interfacial viscosity $\eta_s^* = -10^{-5}i$ Ns/m ($Bq^* = -14i$), at $\omega = 1$ rad/s. Plots at left and right show the in-phase and out-of-phase parts of the velocity amplitude function, respectively.

### *4.2. Interfacial flow profiles*

To illustrate the interfacial flow profiles obtained using the G2 code we plot in Figures 4 (left and right panels, respectively) the interfacial radial profiles of the in-phase and out-of-phase parts of the velocity amplitude function for different values of $Bq^*$ corresponding to purely viscous air/water interfaces. In all cases, the interfaces are sheared at a frequency $\omega = 1$ rad/s. It is clear that the in-phase part of the interfacial radial velocity profile, $\Re(g^*)$, is linear only for $Bq^* \geq 100$ (see Figure 4, left panel) and that the out-of-phase part of the interfacial radial velocity profile, $\Im(g^*)$, is negligible everywhere only for $Bq^* \gg 100$ (see Figure 4, right panel). Moreover, the absolute value of $\Im(g^*)$ is always much smaller than that of $\Re(g^*)$.

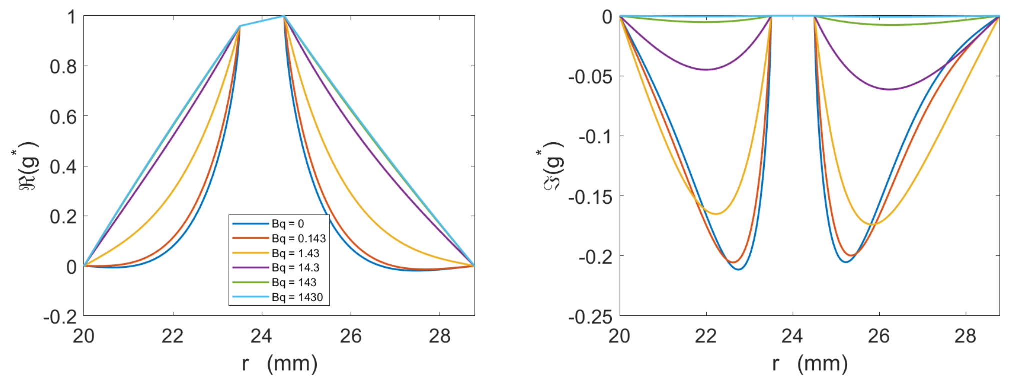


Figure 4: Radial profiles of the in-phase (left panel) and out-of-phase (right panel) parts of the interfacial velocity amplitude function for different values of $Bq^*$. Purely viscous air/water interfaces, sheared at a frequency $\omega = 1$ rad/s.

In Figure 5 (left and right panels, respectively) we show the radial profiles of the in-phase and out-of-phase parts of the interfacial velocity amplitude function for different values of $Bq^*$ corresponding to purely elastic air/water interfaces. In all cases, the interfaces are sheared at a frequency $\omega = 1$ rad/s. Again, the in-phase part of the interfacial radial velocity profile, $\Re(g^*)$, is linear only for $Bq^* \geq 100$ (see Figure 5, left panel) and the interfacial radial velocity profile of $Im(g^*)$ is approximately null everywhere only for $Bq^* \gg 100$ (see Figure 5, right panel). In this case the amplitude of $\Im(g^*)$ may take closer values to those of $\Re(g^*)$ for $Bq^* \sim -1.4i$.

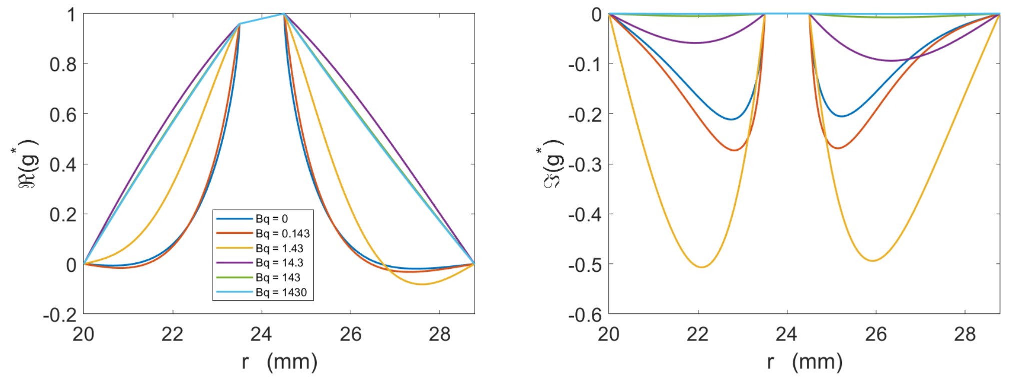


Figure 5: Radial profiles of the in-phase (a) and out-of-phase (b) parts of the interfacial velocity amplitude function for different values of $Bq^*$. Purely elastic air/water interfaces, sheared at a frequency $\omega = 1$ rad/s.

*4.3. Hydrodynamic drag torques*

In Figure 6 we illustrate the dependence of the in-phase (continuous lines) and out-of-phase (dashed lines) parts of the different nondimensional hydrodynamic torques on $Bq = Bq^*_{G1}$, at an air/water interface sheared at $\omega = 1$ rad/s (left panel) and $\omega = 20$ rad/s (right panel). As the torque must be related to the amplitude of the probe's oscillation, what we actually represent is the in-phase and out-of-phase parts of the different contributions to the torque/angle amplitude ratio in Equation 22 of the main text. More explicitly, the contribution from the bulk fluid phases 1 and 2, $AR^*_b = \frac{M^*_1+M^*_2}{\theta_0 e^{i\omega t}}$, the interface contribution, $AR^*_s = \frac{M^*_s}{\theta_0 e^{i\omega t}}$, and the total flow fields contribution, $AR^*_T = AR^*_b + AR^*_s$.

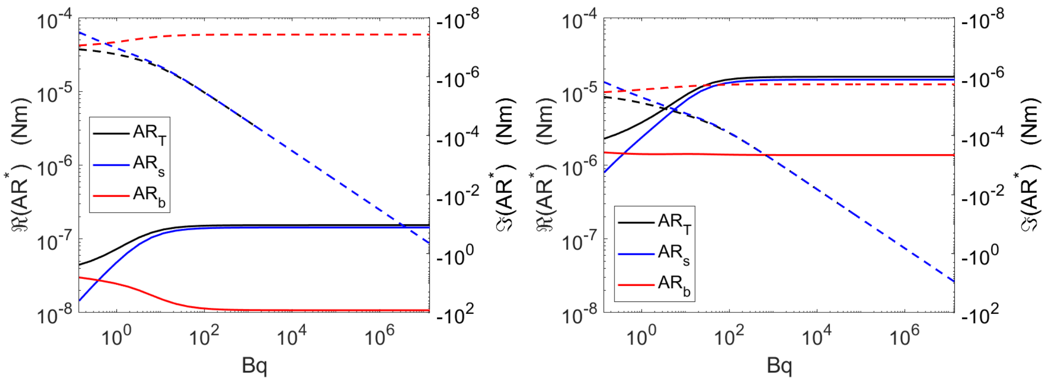


Figure 6: Flow fields contributions to the torque/angle amplitude ratio as a function of the Boussinesq number ($Bq = Bq^*_{G1}$) for purely viscous air/water interfaces $\eta^*_s = \eta_s$). Left panel: $\omega = 1$ rad/s; right panel: $\omega = 20$ rad/s. In-phase (continuous lines) and out-of-phase (dashed lines) parts of the contributions to the torque angle amplitude ratio due to the bulk phases (red), $AR^*_b$, due to the interface (blue), $AR^*_s$, and sum of all contributions of hydrodynamic origin (black), $AR^*_T$.

Two regions with different qualitative behaviors can be recognized in Figure 6 that we will label as low $Bq$ region ($Bq \leq 10$, in the left panel) and high $Bq$ region ($Bq \leq 100$, in the right panel). Trends for the in-phase part of the bulk phases (continuous red lines) and interfacial (continuous blue lines) contributions are similar in both the left and right panels. The in-phase part of the bulk phases contributions decrease upon increasing $Bq$ in the low $Bq$ region, while it levels out in the high $Bq$ region, attaining values $\Re[AR^*_b] \sim 10^{-8}$ Nm (left panel) and $\sim 10^{-6}$ Nm (right panel), respectively. The in-phase part of the interfacial contribution (continuous blue lines) increases

upon increasing $Bq$ in the low $Bq$ region and levels out in the high $Bq$ region, attaining values of $\Re[AR_s^*] \sim 10^{-7}$ Nm (left panel) and $\sim 10^{-5}$ Nm (right panel), respectively.

Something similar happens when considering the out-of-phase parts, although the fact that all out-of-phase parts take negative values has to be kept in mind (a decreasing trend in the graph means an increasing trend of the absolute value of the out-of-phase part). In the low $Bq$ region the absolute values of the out-of-phase parts of the interfacial (respectively, bulk) contribution increases (respectively, decreases). In the high $Bq$ region the out-of-phase part of the bulk contributions levels out, reaching absolute values similar to those of the real part value $|\Im[AR_b^*]| \sim 10^{-8}$ Nm (left panel) and $\sim 10^{-6}$ Nm (right panel), respectively. On the other hand, the absolute value of the out-of-phase part of the interfacial contribution (dashed blue lines) increases, mildly in the low $Bq$ region and strongly in the high $Bq$ one. Consequently, the bulk phases drag dominates the dynamics in the low $Bq$ region and the interfacial drag dominates in the high $Bq$ region, as expected.

### *4.4. Liquid-liquid interfaces*

Finally, we illustrate, very briefly, the performance of the program when applied to liquid-liquid interfaces by considering interfaces in a water/decane system. The parameters for decane at room temperature are, $\rho_2 = 730$ Kg/m$^3$ and $\eta_2 = 8.59 \times 10^{-4}$ Pa·s. Remind that as both bulk subphases above and below the interface are taken into account, the length scale $a = 2L$ must be used in the definition of $Bq^*$.

Figures 7 and 8 show color coded plots of the flow field at the bulk fluid phases for a decane/water interface with interfacial viscosities $\eta_s = 10^7$ Ns/m ($Bq = 0.0768$), and $\eta_s = 10^{-3}$ Ns/m ($Bq = 768$), respectively. Examples of interfacial velocity profiles for different values of $Bq$ for purely viscous interfaces are shown in Figure 9.

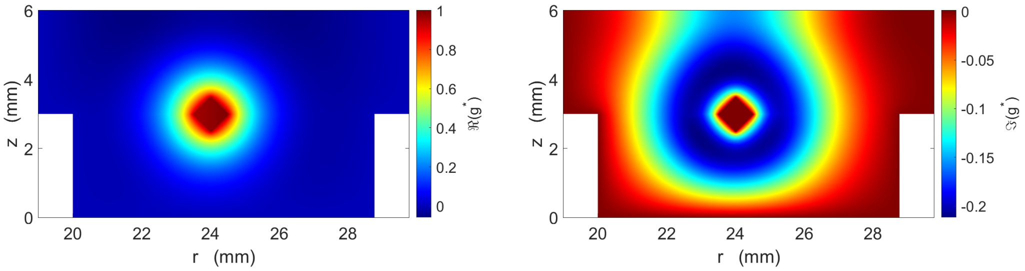


Figure 7: Color coded plot of the flow field at both bulk fluid phases for a purely viscous decane/water interface, with interfacial viscosity $\eta_s = 10^{-7}$ Ns/m ($Bq = 0.0768$), at $\omega = 1$ rad/s. Plots at left and right show the in-phase and out-of-phase parts of the velocity amplitude function, respectively.

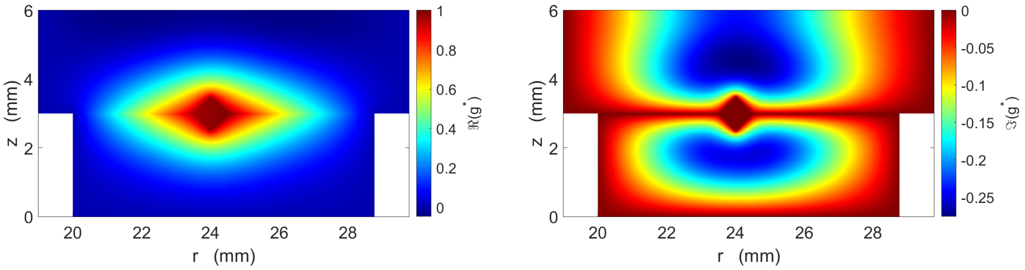


Figure 8: Color coded plot of the flow field at both bulk fluid phases for a purely viscous decane/water interface, with interfacial viscosity $\eta_s = 10^{-3}$ Ns/m ($Bq = 768$), at $\omega = 1$ rad/s. Plots at left and right show the in-phase and out-of-phase parts of the velocity amplitude function, respectively.

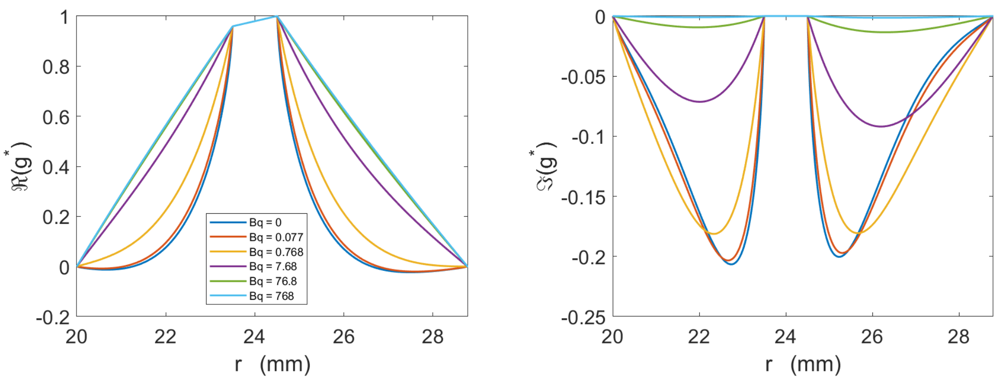


Figure 9: Interfacial radial velocity profiles of the in-phase (left panel) and out-of-phase (right panel) parts of the velocity amplitude function for different values of $Bq^*$. Purely viscous decane/water interfaces, sheared at a frequency $\omega = 1$ rad/s.

We remark that the hydrodynamic model at the basis of both the G1 and G2 software packages does not take into account the unavoidable drag exerted by the upper bulk fluid phase on the (typically 3) spikes that attach the different sections of the ring to the rotor. Hence, the application of both iterative packages to obtain the dynamic moduli or the complex viscosity in the two fluid configuration will be valid only for very high values of the Boussinesq number, where the interfacial drag should dominate the system's dynamics, or shallow upper bulk fluid phases with depth equal to half the diagonal of the ring's diamond cross-section.

## 5. Details of the numerical scheme

### *5.1. Filling the coefficients matrix and the independent terms vector*

We discretize the derivatives by second-order centered finite differences and define the parameter, $A = \frac{1}{\Delta \bar{s}}$, for convenience. Therefore, the first and second order derivatives along the coordinates $\bar{r}$ and $\bar{z}$ reads:

$$\left(\frac{\partial g^*_{j,k}}{\partial \bar{r}}\right)^{(1)}_{j,k} = \left(\frac{\partial g^*_{j,k}}{\partial \bar{r}}\right)^{(2)}_{j,k} = \frac{A}{2}\left(g^*_{j+1,k} - g^*_{j-1,k}\right). \tag{23}$$

$$\left(\frac{\partial g^*_{j,k}}{\partial \bar{z}}\right)^{(1)}_{j,k} = \left(\frac{\partial g^*_{j,k}}{\partial \bar{z}}\right)^{(2)}_{j,k} = \frac{A}{2}\left(g^*_{j,k-1} - g^*_{j,k+1}\right). \tag{24}$$

$$\left(\frac{\partial^2 g^*_{j,k}}{\partial \bar{r}^2}\right)^{(1)}_{j,k} = \left(\frac{\partial^2 g^*_{j,k}}{\partial \bar{r}^2}\right)^{(2)}_{j,k} = A^2\left(g^*_{j+1,k} - 2g^*_{j,k} + g^*_{j-1,k}\right). \tag{25}$$

$$\left(\frac{\partial^2 g^*_{j,k}}{\partial \bar{z}^2}\right)^{(1)}_{j,k} = \left(\frac{\partial^2 g^*_{j,k}}{\partial \bar{z}^2}\right)^{(2)}_{j,k} = A^2\left(g^*_{j,k+1} - 2g^*_{j,k} + g^*_{j,k-1}\right). \tag{26}$$

Rearranging the values of $g^{(1,2)*}_{j,k}$ (Eqs. 25 and 26 of the main text) as a column vector $g^*_\alpha$, of size $(N_1+1)(M+1)+(N_2+1)M$, being

$$\begin{aligned}
& g^*_\alpha = g^*_{j,k}, \quad \text{with} \\
& \alpha = \begin{cases} (k-1)(N_1+1)+j, & \text{if } 1 \le j \le N_1+1\,,\ 1 \le k \le M+1 \\ (k-1)(N_2+1)+j, & \text{if } 1 \le j \le N_2+1\,,\ M+1 \le k \le 2M+1 \end{cases} \\
& \forall \alpha \in \mathbb{Z} \,/\, 1 \le \alpha \le (N_1+1)(M+1)+(N_2+1)M,
\end{aligned} \tag{27}$$

we can write the problem as a linear set of equations

$$\mathbf{A} \cdot \mathbf{g} = \mathbf{b}, \tag{28}$$

where $\mathbf{g} = g^*_\alpha$, $\mathbf{A}$ is the matrix of coefficients (a square sparse matrix of size $(N_1+1)(M+1)+(N_2+1)M \times (N_1+1)(M+1)+(N_2+1)M$, and $\mathbf{b}$ is the vector of independent terms (a null vector except for the nodes at the ring cross section surface).

Note that these expressions are valid for MATLAB code, where indexes $j$ and $k$ run from 1 to $N+1$ and 1 to $M+1$, respectively. In the Python code the expressions are slightly different because index $j$ and $k$ run from 0 to $N$ and from 0 to $M$.

For the nodes internal to the fluid bulk phases (nodes not at a boundary) the discrete Navier-Stokes equation, at node $(j,k)$, takes the form

$$i\frac{Re_1}{A^2}g^*_{j,k} = g^*_{j+1,k} - 4g^*_{j,k} + g^*_{j-1,k} \tag{29}$$
$$+\frac{g^*_{j+1,k} - g^*_{j-1,k}}{2(A\bar{R}_1 + (j-1))} - \frac{g^*_{j,k}}{(A\bar{R}_1 + (j-1))^2} + g^*_{j,k+1} + g^*_{j,k-1}$$
$$\forall j,k \in \mathbb{Z}/2 \leq j \leq N_2, 2 \leq k \leq M. \tag{30}$$

$$i\frac{Re_2}{A^2}g^*_{j,k} = g^*_{j+1,k} - 4g^*_{j,k} + g^*_{j-1,k} \tag{31}$$
$$+\frac{g^*_{j+1,k} - g^*_{j-1,k}}{2(A\bar{R}_2 + (j-1))} - \frac{g^*_{j,k}}{(A\bar{R}_2 + (j-1))^2} + g^*_{j,k+1} + g^*_{j,k-1}$$
$$\forall j,k \in \mathbb{Z}/2 \leq j \leq N_1, M+2 \leq k \leq 2M. \tag{32}$$

Discretized N-S equation, (30) and (32), has been obtained implementing a 5 nodes formula,

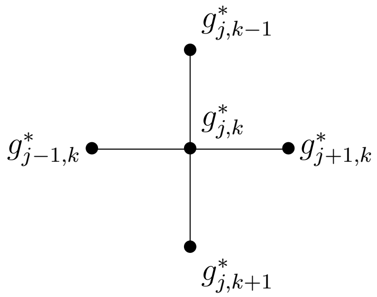


Figure 10: Five nodes scheme for N-S equations

And reorganizing coefficients we obtain the equations for the bulk nodes:

$$g^*_{j,k-1}[1] + g^*_{j-1,k}\left[1 - \frac{1}{2(A\bar{R}_{(1,2)} + (j-1))}\right] + g^*_{j,k}\left[-i\frac{Re_{(1,2)}}{A^2} - 4 - \frac{1}{(A\bar{R}_{(1,2)} + (j-1))^2}\right]$$
$$+ g^*_{j+1,k}\left[1 + \frac{1}{2(A\bar{R}_{(1,2)} + (j-1))}\right] + g^*_{j,k+1}[1] = 0. \tag{33}$$

The boundary conditions at the discretized domain are:

$$g^*_{j,2M+1} = 0 \qquad \text{(ground)}, \qquad \forall k \in \mathbb{Z} \,/\, 2 \leq 1 \leq N_2 + 1, \tag{34}$$

$$g^*_{N+1,k} = g^*_{1,k} = 0 \qquad \text{(walls)}, \qquad \forall j \in \mathbb{Z} \,/\, 1 \leq k \leq M, \tag{35}$$

$$g^*_{1,k} = 0 \qquad \text{(symmetry)}, \qquad \forall j \in \mathbb{Z} \,/\, 1 \leq k \leq \frac{M}{2}, \tag{36}$$

$$g^*_{j,M+1} = \bar{r} \qquad \text{(DWR)}, \tag{37}$$

$$g^*_{j,0} = g^*_{j,2} \qquad \text{(interf libre)}, \qquad \forall k \in \mathbb{Z} \,/\, 2 \leq j \leq N_1. \tag{38}$$

For the upper fluid free boundary condition, extra fictitious nodes are considered. Considering $g^*_{j,0} = g^*_{j,2}$ in the discretized N-S equation:

$$i\frac{Re_2}{A^2} g^*_{j,1} = g^*_{j+1,1} - 4g^*_{j,1} + g^*_{j-1,1} + \frac{g^*_{j+1,1} - g^*_{j-1,1}}{2(A\bar{R}_2 + (j-1))} - \frac{g^*_{j,1}}{(A\bar{R}_2 + (j-1))^2} + 2g^*_{j,2}, \tag{39}$$

$$\forall k \in \mathbb{Z}/2 \leq j \leq N_1.$$

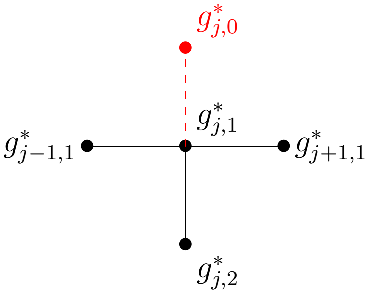


Figure 11: Four nodes scheme for free interface boundary condition. The $g^*_{j,0}$ is highlighted in red color to remark that it is a fictitious node.

Arranging and reorganizing:

$$g^*_{j-1,1}\left[1 - \frac{1}{2(A\bar{R}_2 + (j-1))}\right] + g^*_{j,1}\left[-i\frac{Re_2}{A^2} - 4 - \frac{1}{(A\bar{R}_2 + (j-1))^2}\right] +$$

$$g^*_{j+1,1}\left[1 + \frac{1}{2(A\bar{R}_2 + (j-1))}\right] + g^*_{j,2}\,[2] = 0. \tag{40}$$

To obtain the linear equations for the nodes at the interface we consider Boussinesq-Scriven and implement second order finite differences evaluated at M+1,

- Inner gap

$$
\begin{aligned}
&N\left(g^*_{j+1,M+1}-2g^*_{j,M+1}+g^*_{j-1,M+1}+\frac{g^*_{j+1,M+1}-g^*_{j-1,M+1}}{2(A\bar{R}_2+(j-1))}-\frac{g^*_{j,M+1}}{(A\bar{R}_2+(j-1))^2}\right)\\
&=\frac{1}{2A}\left(\boxed{g^*_{j,M}}-g^*_{j,M+2}\right)-\frac{1}{2AY}\left(g^*_{j,M}-\boxed{g^*_{j,M+2}}\right),\\
&\forall j\in\mathbb{Z}\,/\,2+N_{step}\le j\le N_{step}+NG_1,
\end{aligned}
\tag{41}
$$

- Outer gap

$$
\begin{aligned}
&-N\left(g^*_{j+1,M+1}-2g^*_{j,M+1}+g^*_{j-1,M+1}+\frac{g^*_{j+1,M+1}-g^*_{j-1,M+1}}{2(A\bar{R}_2+(j-1))}-\frac{g^*_{j,M+1}}{(A\bar{R}_2+(j-1))^2}\right)\\
&=\frac{1}{2A}\left(\boxed{g^*_{j,M}}-g^*_{j,M+2}\right)-\frac{1}{2AY}\left(g^*_{j,M}-\boxed{g^*_{j,M+2}}\right),\\
&\forall j\in\mathbb{Z}\,/\,2+N_{step}+N_d+NG_1\le j\le N_{step}+N_d+NG_1+NG_2,
\end{aligned}
\tag{42}
$$

Moreover, we have to write the Navier-Stokes equations for the nodes at the lower and upper bulk phases that are in contact with the interface (with $k=M+1$),

$$
\begin{aligned}
&i\frac{Re_1}{A^2}g^*_{j,k}=g^*_{j+1,M+1}-4g^*_{j,M+1}+g^*_{j-1,M+1}+\frac{g^*_{j+1,M+1}-g^*_{j-1,M+1}}{2(A\bar{R}_2+(j-1))}\\
&-\frac{g^*_{j,M+1}}{(A\bar{R}_2+(j-1))^2}+g^*_{j,M+2}+\boxed{g^*_{j,M}},\forall j\in\mathbb{Z}\,/\,2+N_{step}\le j\le M_{step}+NG_1\\
&\quad\text{and}\quad 2+N_{step}+N_d+NG_1\le j\le N_{step}+N_d+NG_1+NG_2.
\end{aligned}
\tag{43}
$$

$$
\begin{aligned}
&i\frac{Re_2}{A^2}g^*_{j,k}=g^*_{j+1,M+1}-4g^*_{j,M+1}+g^*_{j-1,M+1}+\frac{g^*_{j+1,M+1}-g^*_{j-1,M+1}}{2(A\bar{R}_2+(j-1))}\\
&-\frac{g^*_{j,M+1}}{(A\bar{R}_2+(j-1))^2}+\boxed{g^*_{j,M+2}}+g^*_{j,M},\forall j\in\mathbb{Z}\,/\,2+N_{step}\le j\le N_{step}+NG_1\\
&\text{and}\quad 2+N_{step}+N_d+NG_1\le j\le N_{step}+N_d+NG_1+NG_2.
\end{aligned}
\tag{44}
$$

Next, we have to combine the Boussinesq-Scriven equations for the inner and outer gaps, Equations (41) and (42), respectively, with the Navier-Stokes equations at the lower and upper bulk phases, Equations (43) and (44), respectively. Solving for $g^*_{j,M}$ and $g^*_{j,M+2}$ in Equations (43) and (44), respectively, and substituting their expressions in Equations (41) and (42) for the inner and outer gaps, yield the linearized equations for the interfacial nodes at both sides of the ring, resulting in a 5 node formula.

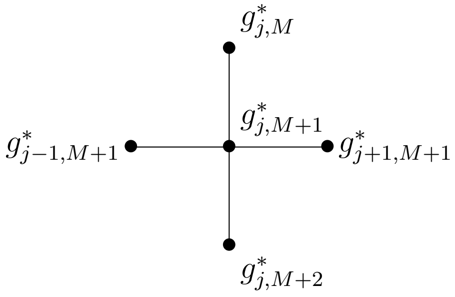


Figure 12: Five nodes scheme for interface boundary condition

Arranging and reorganizing:

- Inner

$$\begin{aligned}
&g^*_{j,M}\left[\frac{1}{AY}\right] + g^*_{j-1,M+1}\left[\left(1-\frac{1}{2(A\bar{R}_2+(j-1))}\right)\left(N+\frac{1}{2A}\left(1+\frac{1}{Y}\right)\right)\right]\\
&+ g^*_{j,M+1}\left[-N\left(2+\frac{1}{(A\bar{R}_2+(j-1))^2}\right)-\left(\frac{1}{2A}\right)\left(i\frac{Re_1}{A^2}+4+\frac{1}{(A\bar{R}_2+(j-1))^2}\right.\right.\\
&\left.\left.-\left(\frac{1}{Y}\right)\left(i\frac{Re_2}{A^2}+4+\frac{1}{(A\bar{R}_2+(j-1))^2}\right)\right)\right]\\
&+ g^*_{j+1,M+1}\left[\left(1+\frac{1}{2(A\bar{R}_2+(j-1))}\right)\left(N+\frac{1}{2A}\left(1+\frac{1}{Y}\right)\right)\right] + g^*_{j,M+2}\left[\frac{1}{A}\right]=0,\\
&\forall j\in\mathbb{Z}\,/\,2+N_{step}\le j\le N_{step}+NG_1. \qquad (45)
\end{aligned}$$

- Outer

$$
\begin{aligned}
&g^*_{j,M}\left[\frac{1}{AY}\right]+g^*_{j-1,M+1}\left[\left(1-\frac{1}{2(A\bar{R}_2+(j-1))}\right)\left(-N+\frac{1}{2A}\left(1+\frac{1}{Y}\right)\right)\right]\\
&+g^*_{j,M+1}\left[N\left(2+\frac{1}{(A\bar{R}_2+(j-1))^2}\right)-\left(\frac{1}{2A}\right)\left(i\frac{Re_1}{A^2}+4+\frac{1}{(A\bar{R}_2+(j-1))^2}\right.\right.\\
&\left.\left.-\left(\frac{1}{Y}\right)\left(i\frac{Re_2}{A^2}+4+\frac{1}{(A\bar{R}_2+(j-1))^2}\right)\right)\right]\\
&+g^*_{j+1,M+1}\left[\left(1+\frac{1}{2(A\bar{R}_2+(j-1))}\right)\left(-N+\frac{1}{2A}\left(1+\frac{1}{Y}\right)\right)\right]+g^*_{j,M+2}\left[\frac{1}{A}\right]=0,\\
&\forall j\in\mathbb{Z}\,/\,2+N_{step}+N_d+NG_1\le j\le N_{step}+N_d+NG_1+NG_2.
\end{aligned}
\tag{46}
$$
